# Supplementary material for: MultiLegalPile: A 689GB Multilingual Legal Corpus
Source: arXiv:2306.02069 source file (2024-05-19)
Supplement: Supplementary file 1 [file additional_appendices.tex]

\begin{table*}[!ht]
    \fontsize{9pt}{9pt}\selectfont
    \centering
    \caption{Eurlex Resources}
    \begin{tabular}{lrrrr}
\toprule
    \textbf{Source} &  \textbf{Size (MB)} &  \textbf{Words} &  \textbf{Documents} &  \textbf{Words/Document} \\
\midrule
           all\_all &              180668 &     12106556233 &             8306749 &                     1457 \\
       all\_caselaw &               34939 &      3413551598 &             2487794 &                     1372 \\
      all\_decision &               28519 &      1698585620 &             1267402 &                     1340 \\
     all\_directive &                4786 &       368577940 &              104187 &                     3537 \\
        all\_intagr &               11421 &       743271516 &              274485 &                     2707 \\
      all\_proposal &               26526 &      2087989530 &              702392 &                     2972 \\
all\_recommendation &                1886 &       164979037 &               80277 &                     2055 \\
    all\_regulation &               72590 &      3629600992 &             3390212 &                     1070 \\
            bg\_all &                7819 &       398067053 &              348691 &                     1141 \\
        bg\_caselaw &                1588 &       109749174 &              104434 &                     1050 \\
       bg\_decision &                1248 &        58817972 &               54075 &                     1087 \\
      bg\_directive &                 263 &        15731608 &                4388 &                     3585 \\
         bg\_intagr &                 603 &        31292848 &               11581 &                     2702 \\
       bg\_proposal &                1083 &        60674956 &               29251 &                     2074 \\
 bg\_recommendation &                  89 &         5588991 &                3321 &                     1682 \\
     bg\_regulation &                2943 &       116211504 &              141641 &                      820 \\
            cs\_all &                8360 &       471961631 &              449793 &                     1049 \\
        cs\_caselaw &                1163 &       110005022 &              104519 &                     1052 \\
       cs\_decision &                1102 &        58921128 &               54075 &                     1089 \\
      cs\_directive &                 186 &        13951134 &                4388 &                     3179 \\
         cs\_intagr &                 449 &        28106332 &               11581 &                     2426 \\
       cs\_proposal &                 840 &        61838692 &               29252 &                     2113 \\
 cs\_recommendation &                  64 &         5416549 &                3323 &                     1630 \\
     cs\_regulation &                4557 &       193722774 &              242655 &                      798 \\
            da\_all &                8932 &       671484862 &              332500 &                     2019 \\
        da\_caselaw &                1746 &       185589641 &               88234 &                     2103 \\
       da\_decision &                1356 &        89498535 &               54085 &                     1654 \\
      da\_directive &                 207 &        17525792 &                4388 &                     3994 \\
         da\_intagr &                 506 &        35596169 &               11582 &                     3073 \\
       da\_proposal &                1399 &       119759476 &               29257 &                     4093 \\
 da\_recommendation &                 100 &         9463897 &                3352 &                     2823 \\
     da\_regulation &                3618 &       214051352 &              141602 &                     1511 \\
            de\_all &                9607 &       695512401 &              348290 &                     1996 \\
        de\_caselaw &                1930 &       193232441 &              104228 &                     1853 \\
       de\_decision &                1449 &        93688222 &               53980 &                     1735 \\
      de\_directive &                 218 &        17337760 &                4385 &                     3953 \\
         de\_intagr &                 531 &        36791153 &               11580 &                     3177 \\
       de\_proposal &                1556 &       126987454 &               29219 &                     4346 \\
 de\_recommendation &                 109 &         9608034 &                3318 &                     2895 \\
     de\_regulation &                3813 &       217867337 &              141580 &                     1538 \\
            el\_all &               12469 &       696216541 &              349667 &                     1991 \\
        el\_caselaw &                2951 &       202027703 &              105138 &                     1921 \\
       el\_decision &                1823 &        94919886 &               54150 &                     1752 \\
      el\_directive &                 321 &        19411959 &                4390 &                     4421 \\
         el\_intagr &                 701 &        38965777 &               11584 &                     3363 \\
       el\_proposal &                2085 &       128005737 &               29290 &                     4370 \\
 el\_recommendation &                 145 &         9344866 &                3357 &                     2783 \\
     el\_regulation &                4443 &       203540613 &              141758 &                     1435 \\
            en\_all &                9217 &       769465561 &              348641 &                     2207 \\
        en\_caselaw &                1846 &       222891827 &              104422 &                     2134 \\
       en\_decision &                1504 &       114626013 &               54054 &                     2120 \\
      en\_directive &                 204 &        18860876 &                4388 &                     4298 \\
         en\_intagr &                 499 &        39029843 &               11581 &                     3370 \\
       en\_proposal &                1538 &       140781768 &               29242 &                     4814 \\
 en\_recommendation &                  97 &        10091809 &                3320 &                     3039 \\
     en\_regulation &                3530 &       223183425 &              141634 &                     1575 \\
            es\_all &                8588 &       725125274 &              348443 &                     2081 \\
        es\_caselaw &                1870 &       220621730 &              104312 &                     2115 \\
       es\_decision &                1334 &        98163499 &               54001 &                     1817 \\
      es\_directive &                 221 &        21484479 &                4385 &                     4899 \\
         es\_intagr &                 516 &        41841805 &               11581 &                     3612 \\
       es\_proposal &                1366 &       133674486 &               29224 &                     4574 \\
 es\_recommendation &                  82 &         8864018 &                3319 &                     2670 \\
     es\_regulation &                3199 &       200475257 &              141621 &                     1415 \\
            et\_all &                6090 &       328068754 &              349615 &                      938 \\
        et\_caselaw &                1074 &        93096396 &              105111 &                      885 \\
       et\_decision &                1069 &        50752324 &               54159 &                      937 \\
      et\_directive &                 177 &        11555930 &                4390 &                     2632 \\
         et\_intagr &                 436 &        24018147 &               11584 &                     2073 \\
       et\_proposal &                 810 &        51600852 &               29283 &                     1762 \\
 et\_recommendation &                  61 &         4451369 &                3355 &                     1326 \\
     et\_regulation &                2464 &        92593736 &              141733 &                      653 \\
            fi\_all &                7346 &       404265224 &              349633 &                     1156 \\
        fi\_caselaw &                1596 &       126525296 &              105119 &                     1203 \\
       fi\_decision &                1227 &        59659475 &               54163 &                     1101 \\
      fi\_directive &                 204 &        12766491 &                4389 &                     2908 \\
         fi\_intagr &                 463 &        25392311 &               11584 &                     2192 \\
       fi\_proposal &                1075 &        69198401 &               29288 &                     2362 \\
 fi\_recommendation &                  73 &         5070392 &                3356 &                     1510 \\
     fi\_regulation &                2707 &       105652858 &              141734 &                      745 \\
            fr\_all &                9937 &       828959218 &              348295 &                     2380 \\
        fr\_caselaw &                2158 &       246262666 &              104228 &                     2362 \\
       fr\_decision &                1473 &       108648744 &               53981 &                     2012 \\
      fr\_directive &                 222 &        20308801 &                4385 &                     4631 \\
         fr\_intagr &                 536 &        41986012 &               11580 &                     3625 \\
       fr\_proposal &                1592 &       149134298 &               29218 &                     5104 \\
 fr\_recommendation &                 112 &        11510415 &                3318 &                     3469 \\
     fr\_regulation &                3845 &       251108282 &              141585 &                     1773 \\
            ga\_all &                1028 &        65030095 &              349778 &                      185 \\
        ga\_caselaw &                  11 &          696305 &              105205 &                        6 \\
       ga\_decision &                  87 &         4415457 &               54189 &                       81 \\
      ga\_directive &                  18 &         1512027 &                4390 &                      344 \\
         ga\_intagr &                  19 &         1820723 &               11586 &                      157 \\
       ga\_proposal &                 289 &        26106889 &               29298 &                      891 \\
 ga\_recommendation &                  10 &          902390 &                3361 &                      268 \\
     ga\_regulation &                 594 &        29576304 &              141749 &                      208 \\
            hr\_all &                4594 &       258816068 &              348691 &                      742 \\
        hr\_caselaw &                 617 &        62432734 &              104434 &                      597 \\
       hr\_decision &                 596 &        31911903 &               54075 &                      590 \\
      hr\_directive &                 156 &        10855913 &                4388 &                     2474 \\
         hr\_intagr &                 450 &        24962086 &               11581 &                     2155 \\
       hr\_proposal &                 552 &        33437815 &               29251 &                     1143 \\
 hr\_recommendation &                  40 &         3612247 &                3321 &                     1087 \\
     hr\_regulation &                2183 &        91603370 &              141641 &                      646 \\
            hu\_all &                6653 &       375253894 &              349605 &                     1073 \\
        hu\_caselaw &                1278 &       110179375 &              105144 &                     1047 \\
       hu\_decision &                1147 &        57108172 &               54156 &                     1054 \\
      hu\_directive &                 200 &        13568304 &                4389 &                     3091 \\
         hu\_intagr &                 470 &        27258501 &               11586 &                     2352 \\
       hu\_proposal &                 912 &        60882750 &               29291 &                     2078 \\
 hu\_recommendation &                  70 &         5312868 &                3357 &                     1582 \\
     hu\_regulation &                2576 &       100943924 &              141682 &                      712 \\
            it\_all &                9586 &       768605772 &              333631 &                     2303 \\
        it\_caselaw &                1889 &       206117726 &               89560 &                     2301 \\
       it\_decision &                1445 &       102848859 &               53983 &                     1905 \\
      it\_directive &                 217 &        19687773 &                4385 &                     4489 \\
         it\_intagr &                 528 &        40134330 &               11580 &                     3465 \\
       it\_proposal &                1533 &       140713925 &               29218 &                     4816 \\
 it\_recommendation &                 109 &        10923431 &                3318 &                     3292 \\
     it\_regulation &                3865 &       248179728 &              141587 &                     1752 \\
            lt\_all &                6400 &       364361783 &              200565 &                     1816 \\
        lt\_caselaw &                1137 &       101808706 &              105477 &                      965 \\
       lt\_decision &                1096 &        55850308 &               21990 &                     2539 \\
      lt\_directive &                 185 &        13078983 &                3239 &                     4037 \\
         lt\_intagr &                 452 &        27009631 &                7481 &                     3610 \\
       lt\_proposal &                 850 &        58553579 &               29272 &                     2000 \\
 lt\_recommendation &                  64 &         5121089 &                3363 &                     1522 \\
     lt\_regulation &                2617 &       102939487 &               29743 &                     3460 \\
            lv\_all &                6349 &       363239195 &              349919 &                     1038 \\
        lv\_caselaw &                1153 &       103456811 &              105242 &                      983 \\
       lv\_decision &                1103 &        55512944 &               54224 &                     1023 \\
      lv\_directive &                 186 &        13023024 &                4392 &                     2965 \\
         lv\_intagr &                 452 &        26693107 &               11630 &                     2295 \\
       lv\_proposal &                  96 &        58176216 &               29298 &                     1985 \\
 lv\_recommendation &                  64 &         5074494 &                3361 &                     1509 \\
     lv\_regulation &                2545 &       101302599 &              141772 &                      714 \\
            mt\_all &                6540 &       367834815 &              350292 &                     1050 \\
        mt\_caselaw &                1164 &       100423543 &              105479 &                      952 \\
       mt\_decision &                1109 &        55239141 &               54280 &                     1017 \\
      mt\_directive &                 203 &        14355266 &                4392 &                     3268 \\
         mt\_intagr &                 470 &        27701991 &               11675 &                     2372 \\
       mt\_proposal &                 878 &        59749277 &               29274 &                     2041 \\
 mt\_recommendation &                  65 &         5039600 &                3363 &                     1498 \\
     mt\_regulation &                2650 &       105325997 &              141829 &                      742 \\
            nl\_all &                9586 &       770312808 &              349407 &                     2204 \\
        nl\_caselaw &                1847 &       206271837 &              105005 &                     1964 \\
       nl\_decision &                1456 &       104060901 &               54152 &                     1921 \\
      nl\_directive &                 217 &        19529361 &                4388 &                     4450 \\
         nl\_intagr &                 529 &        40247634 &               11584 &                     3474 \\
       nl\_proposal &                1540 &       141258274 &               29279 &                     4824 \\
 nl\_recommendation &                 111 &        11002405 &                3355 &                     3279 \\
     nl\_regulation &                3886 &       247942396 &              141644 &                     1750 \\
            pl\_all &                6677 &       406648795 &              350349 &                     1160 \\
        pl\_caselaw &                1231 &       115824759 &              105479 &                     1098 \\
       pl\_decision &                1125 &        60407576 &               54287 &                     1112 \\
      pl\_directive &                 197 &        14672157 &                4392 &                     3340 \\
         pl\_intagr &                 466 &        28543668 &               11680 &                     2443 \\
       pl\_proposal &                 886 &        64728230 &               29317 &                     2207 \\
 pl\_recommendation &                  68 &         5769893 &                3363 &                     1715 \\
     pl\_regulation &                2703 &       116702512 &              141831 &                      822 \\
            pt\_all &                8450 &       675152149 &              348449 &                     1937 \\
        pt\_caselaw &                1763 &       198084937 &              104312 &                     1898 \\
       pt\_decision &                1327 &        93278293 &               54007 &                     1727 \\
      pt\_directive &                 217 &        19831549 &                4385 &                     4522 \\
         pt\_intagr &                 504 &        37999753 &               11581 &                     3281 \\
       pt\_proposal &                1361 &       127461782 &               29224 &                     4361 \\
 pt\_recommendation &                  81 &         8396661 &                3319 &                     2529 \\
     pt\_regulation &                3197 &       190099174 &              141621 &                     1342 \\
            ro\_all &                6315 &       415038571 &              350300 &                     1184 \\
        ro\_caselaw &                1110 &       114780999 &              105516 &                     1087 \\
       ro\_decision &                1047 &        59479553 &               54281 &                     1095 \\
      ro\_directive &                 206 &        16101628 &                4392 &                     3666 \\
         ro\_intagr &                 481 &        31497000 &               11675 &                     2697 \\
       ro\_proposal &                 805 &        62130419 &               29274 &                     2122 \\
 ro\_recommendation &                  63 &         5977913 &                3363 &                     1777 \\
     ro\_regulation &                2603 &       125071059 &              141799 &                      882 \\
            sk\_all &                6484 &       392235510 &              350570 &                     1118 \\
        sk\_caselaw &                1160 &       110125141 &              105608 &                     1042 \\
       sk\_decision &                1111 &        59576875 &               54349 &                     1096 \\
      sk\_directive &                 188 &        14132755 &                4393 &                     3217 \\
         sk\_intagr &                 458 &        28298155 &               11676 &                     2423 \\
       sk\_proposal &                 859 &        63726047 &               29290 &                     2175 \\
 sk\_recommendation &                  66 &         5654790 &                3364 &                     1680 \\
     sk\_regulation &                2642 &       110721747 &              141890 &                      780 \\
            sl\_all &                6222 &       394814289 &              350574 &                     1126 \\
        sl\_caselaw &                1071 &       111238184 &              105608 &                     1053 \\
       sl\_decision &                1075 &        59454906 &               54349 &                     1093 \\
      sl\_directive &                 176 &        13908097 &                4393 &                     3165 \\
         sl\_intagr &                 441 &        28239078 &               11676 &                     2418 \\
       sl\_proposal &                 812 &        63391970 &               29290 &                     2164 \\
 sl\_recommendation &                  62 &         5628775 &                3364 &                     1673 \\
     sl\_regulation &                2585 &       112953279 &              141894 &                      796 \\
            sv\_all &                7419 &       500085970 &              351051 &                     1424 \\
        sv\_caselaw &                1585 &       162108645 &              105980 &                     1529 \\
       sv\_decision &                1213 &        71744934 &               54357 &                     1319 \\
      sv\_directive &                 195 &        15386273 &                4393 &                     3502 \\
         sv\_intagr &                 463 &        29845462 &               11676 &                     2556 \\
       sv\_proposal &                1059 &        86016237 &               29292 &                     2936 \\
 sv\_recommendation &                  79 &         7152141 &                3366 &                     2124 \\
     sv\_regulation &                2825 &       127832278 &              141987 &                      900 \\
\bottomrule
\end{tabular}
\caption{Eurlex Resources: The statistics.}
    \label{tab:eurlex_resources}
\end{table*}
